# Supplementary material for: Statistical Inference Based on a New Weighted Likelihood Approach
Source: arXiv:1610.07949 source file (2019-08-27)
Supplement: Supplementary file 1 [file ESM1.pdf]

**Advances in Statistical Analysis manuscript No.**
(will be inserted by the editor)

# Statistical Inference Based on a New Weighted Likelihood Approach

# Supplementary Materials

**Suman Majumder · Adhidev Biswas · Tania Roy · Subir Kumar Bhandari · Ayanendranath Basu**

Received: date / Accepted: date

## 1 Tables of Estimates for different values of $p$ for the Data Examples

### 1.1 Drosophila Data

Table 1: Comparison of estimates of the mean for Drosophila data under different values of $p$

| Method | MLE | MLE-D | $WLE_1$ | | | $WLE_2$ | | |
|---|---|---|---|---|---|---|---|---|
| $p$ | - | - | 0.1 | 0.25 | 0.5 | 0.1 | 0.25 | 0.5 |
| $\hat{\theta}$ | 3.0588 | 0.3939 | 0.3937 | 0.3937 | 0.3938 | 0.3937 | 0.3937 | 0.3938 |

Table 2: Comparison of estimates of the mean for Newcomb speed of light data under different values of $p$

| Method | MLE | MLE-D | $WLE_1$ | | | $WLE_3$ | | |
|---|---|---|---|---|---|---|---|---|
| $p$ | - | - | 0.1 | 0.25 | 0.5 | 0.1 | 0.25 | 0.5 |
| $\hat{\mu}$ | 6.2121 | 27.75 | 27.7595 | 27.7596 | 27.7596 | 27.7898 | 27.7909 | 27.7917 |
| $\hat{\sigma}^2$ | 113.7126 | 25.4375 | 25.2917 | 25.2919 | 25.2927 | 24.5441 | 24.5458 | 24.5567 |

Table 3: Comparison of estimates of the mean for Melbourne rainfall data under different values of $p$

| Method | MLE | MLE-D | $WLE_1$ | | | $WLE_2$ | | |
|---|---|---|---|---|---|---|---|---|
| $p$ | - | - | 0.1 | 0.25 | 0.5 | 0.1 | 0.25 | 0.5 |
| $\hat{\theta}$ | 4.4968 | 3.6403 | 3.6338 | 3.6416 | 3.6437 | 3.6320 | 3.6417 | 3.6443 |

Suman Majumder
Department of Statistics, North Carolina State University, 2311 Stinson Drive, Raleigh, NC 27695, USA
Tel: +1-919-633-0988
E-mail: smajumd2@ncsu.edu

Adhidev Biswas, Subir Kumar Bhandari, Ayanendranath Basu
Interdisciplinary Statistical Research Unit, Indian Statistical Institute, 203 B.T. Road, Kolkata-700108, India
E-mail: adhidevbiswas@gmail.com, subir@isical.ac.in, ayanbasu@isical.ac.in

Tania Roy
Department of Statistics, UC Davis, One Shields Avenue, Davis, CA 95616, USA
E-mail: tania112358@gmail.com

## 2 Determination of First Order Influence Function of the Estimator

### 2.1 Fisher Consistency

**Lemma 1** *The proposed weighted likelihood estimator is Fisher-consistent.*

*Proof* The weighted likelihood functional $T(G)$ is defined as a solution to the equation

$$\int_{\mathscr{X}} H(\tau_{G,t}(x))u_t(x)dG(x) = 0, \tag{1}$$

where $\tau_{G,t}(\cdot)$ is defined as

$$\tau_{G,t}(x) = \begin{cases} \dfrac{G(x)}{F_t(x)} - 1, & \text{if } 0 < F_t(x) \leqslant 1/2 \\ \dfrac{\bar{G}(x)}{S_t(x)} - 1, & \text{if } 1/2 < F_t(x) < 1. \end{cases}$$

It has been proved in Section 4 of this article that the weighted likelihood estimating equation

$$\sum_{i=1}^{n} w_\theta(X_i)u_\theta(X_i) = 0 \tag{2}$$

and the maximum likelihood estimating equation

$$\sum_{i=1}^{n} u_\theta(X_i) = 0 \tag{3}$$

are asymptotically equivalent under some regularity conditions. Using this result and the fact that the expectation of likelihood score function under the model is zero (under similar regularity conditions to be given in Section 4) we assert that

$$\mathbb{E}_\theta[H(\tau_{F_\theta,\theta}(X))u_\theta(X)] = 0,$$

which establishes our claim and proves the result. □

### 2.2 Form of the Influence Function

**Theorem 1** *The influence function of the proposed weighted likelihood estimator is given by*

$$T'(y) = \frac{\partial}{\partial \varepsilon}\theta_\varepsilon\bigg|_{\varepsilon=0} = D^{-1}N, \tag{4}$$

*where*

$$\begin{aligned} D = &\Bigg[\int_{\mathscr{X}_1} H'(\tau(x))u_{\theta_g}(x)\frac{\nabla F_{\theta_g}(x)}{F_{\theta_g}(x)}(\tau(x)+1)dG(x) \\ &+ \int_{\mathscr{X}_2} H'(\tau(x))u_{\theta_g}(x)\frac{\nabla S_{\theta_g}(x)}{S_{\theta_g}(x)}(\tau(x)+1)dG(x) \\ &+ \int H(\tau(x))\nabla(-u_{\theta_g}(x))dG(x)\Bigg], \\ N = &\left[H(\tau(y))u_{\theta_g}(y) + \int_{\mathscr{X}_1} H'(\tau(x))\Delta_y(x)\frac{u_{\theta_g}(x)}{F_{\theta_g}(x)}dG(x)\right] \\ &+ \int_{\mathscr{X}_2} H'(\tau(x))\bar{\Delta}_y(x)\frac{u_{\theta_g}(x)}{S_{\theta_g}(x)}dG(x) \\ &- \int H'(\tau(x))(\tau(x)+1)u_{\theta_g}(x)dG(x)\Bigg], \end{aligned}$$

*with* $\theta_g = T(G)$, $\theta_\varepsilon$ *the functional corresponding to the contaminated distribution*

$$G_\varepsilon(x) = (1-\varepsilon)G(x) + \varepsilon\Lambda_y(x), \tag{5}$$

*with* $\Lambda_y(x)$ *being the distribution function of the random variable* $\chi_y$ *which is degenerate at y.* $\mathscr{X}_1 = \{x \in \mathscr{X} : F_\theta(x) \leqslant 1/2\}$ *and* $\mathscr{X}_2 = \{x \in \mathscr{X} : F_\theta(x) > 1/2\}$ *and* $\mathscr{X}$ *being the support of the distribution. Note that* $\mathscr{X}_1$ *and* $\mathscr{X}_2$ *are disjoint and* $\mathscr{X} = \mathscr{X}_1 \cup \mathscr{X}_2$. *When the true distribution G belongs to the model, then* $G(x) = F_\theta(x)$ *for some* $\theta \in \Theta$ *and the influence function takes the simple form*

$$T'(y) = \left[\int -\nabla u_\theta(x) dF_\theta(x)\right]^{-1} u_\theta(y) = I^{-1}(\theta)u_\theta(y),$$

*which is the same as the influence function of the maximum likelihood estimator.*

*Proof* Let our residual function be defined as:

$$\tau_\varepsilon(x) = \begin{cases} \dfrac{G_\varepsilon(x)}{F_{\theta_\varepsilon}(x)} - 1, & \text{if } 0 < F_{\theta_\varepsilon}(x) \leqslant 1/2, \\ \dfrac{\bar{G}_\varepsilon(x)}{S_{\theta_\varepsilon}(x)} - 1, & \text{if } 1/2 < F_{\theta_\varepsilon}(x) < 1, \end{cases}$$

where $\bar{G}_\varepsilon(x) = (1-\varepsilon)\bar{G}(x) + \varepsilon\bar{\Delta}_y(x)$. We want to differentiate the weighted likelihood estimating equation

$$\int_{\mathscr{X}} H(\tau_\varepsilon(x)) u_{\theta_\varepsilon}(x) dG_\varepsilon(x) = 0 \tag{6}$$

with respect to $\varepsilon$. We assume that the the underlying distribution has a probability density function $g$. Let $\zeta_\varepsilon$ be the median of the contaminated distribution. We define the two sets

$$\mathscr{X}_{1,\varepsilon} = (a, \zeta_\varepsilon] \text{ and } \mathscr{X}_{2,\varepsilon} = (\zeta_\varepsilon, b),$$

where $a < b$ and both of them can either be finite or infinite. Clearly, $\mathscr{X} = \mathscr{X}_{1,\varepsilon} \cup \mathscr{X}_{2,\varepsilon} = (a,b)$. Hence, the right side of the above expression can be written as

$$\frac{\partial}{\partial\varepsilon}\int_a^{\zeta_\varepsilon} H(\tau_\varepsilon(x)) u_{\theta_\varepsilon}(x) g_\varepsilon(x) dx + \frac{\partial}{\partial\varepsilon}\int_{\zeta_\varepsilon}^{b} H(\tau_\varepsilon(x)) u_{\theta_\varepsilon}(x) g_\varepsilon(x) dx.$$

Now, applying Leibniz integral rule, we get the above expression to be

$$\begin{aligned} &\int_a^{\zeta_\varepsilon} \frac{\partial}{\partial\varepsilon}(H(\tau_\varepsilon(x)) u_{\theta_\varepsilon}(x) g_\varepsilon(x)) dx + H(\tau_\varepsilon(\zeta_\varepsilon)) u_{\theta_\varepsilon}(\zeta_\varepsilon) g_\varepsilon(\zeta_\varepsilon) \left(\frac{\partial}{\partial\varepsilon}\zeta_\varepsilon\right) \\ &+ \int_{\zeta_\varepsilon}^{b} \frac{\partial}{\partial\varepsilon}(H(\tau_\varepsilon(x)) u_{\theta_\varepsilon}(x) g_\varepsilon(x)) dx - H(\tau_\varepsilon(\zeta_\varepsilon)) u_{\theta_\varepsilon}(\zeta_\varepsilon) g_\varepsilon(\zeta_\varepsilon) \left(\frac{\partial}{\partial\varepsilon}\zeta_\varepsilon\right), \end{aligned}$$

which leads to the equation

$$\begin{aligned} &\int_{\mathscr{X}_{1,\varepsilon}} H'(\tau_\varepsilon(x)) \tau'_\varepsilon(x) u_{\theta_\varepsilon}(x) dG_\varepsilon(x) + \theta'_\varepsilon \left[\int_{\mathscr{X}_{1,\varepsilon}} H(\tau_\varepsilon(x)) \nabla u_{\theta_\varepsilon}(x) dG_\varepsilon(x)\right] \\ &\int_{\mathscr{X}_{1,\varepsilon}} H(\tau_\varepsilon(x)) u_{\theta_\varepsilon}(x) d(\Delta_y - G)(x) + \int_{\mathscr{X}_{2,\varepsilon}} H'(\tau_\varepsilon(x)) \tau'_\varepsilon(x) u_{\theta_\varepsilon}(x) dG_\varepsilon(x) + \\ &\theta'_\varepsilon \left[\int_{\mathscr{X}_{2,\varepsilon}} H(\tau_\varepsilon(x)) \nabla u_{\theta_\varepsilon}(x) dG_\varepsilon(x)\right] + \int_{\mathscr{X}_{2,\varepsilon}} H(\tau_\varepsilon(x)) u_{\theta_\varepsilon}(x) d(\Delta_y - G)(x) = 0. \end{aligned} \tag{7}$$

For $x \in \mathscr{X}_{1,\varepsilon}$, note that

$$\tau'_\varepsilon(x)|_{\varepsilon=0} = \frac{1}{F_{\theta_g}(x)}\left[\Delta_y(x) - G(x) - \frac{\nabla F_{\theta_g}(x)}{F_{\theta_g}(x)} T'(y) G(x)\right],$$

and for $x \in \mathscr{X}_{2,\varepsilon}$, we have,

$$\tau'_\varepsilon(x)|_{\varepsilon=0} = \frac{1}{S_{\theta_g}(x)}\left[\bar{\Delta}_y(x) - \bar{G}(x) - \frac{\nabla S_{\theta_g}(x)}{S_{\theta_g}(x)} T'(y)\bar{G}(x)\right],$$

where $T'(y) \equiv \theta'_\varepsilon|_{\varepsilon=0}$ is the required influence function. When the expression for $\tau'_\varepsilon(x)|_{\varepsilon=0}$ is substituted in the above equation (7), we get,

$$\begin{aligned}
&T'(y)\Bigg[\int_{\mathscr{X}_1} H'(\tau(x))u_{\theta_g}(x)\frac{\nabla F_{\theta_g}(x)}{F_{\theta_g}(x)}\frac{G(x)}{F_{\theta_g}(x)}dG(x) + \\
&\int_{\mathscr{X}_2} H'(\tau(x))u_{\theta_g}(x)\frac{\nabla S_{\theta_g}(x)}{S_{\theta_g}(x)}\frac{\bar{G}(x)}{S_{\theta_g}(x)}dG(x) - \int H(\tau(x))\nabla u_{\theta_g}(x)dG(x)\Bigg] \\
&= H(\tau(y))u_{\theta_g}(y) + \int_{\mathscr{X}_1} H'(\tau(x))[\Delta_y - G](x)\frac{u_{\theta_g}(x)}{F_{\theta_g}(x)}dG(x) \\
&\quad + \int_{\mathscr{X}_2} H'(\tau(x))[\bar{\Delta}_y - \bar{G}](x)\frac{u_{\theta_g}(x)}{S_{\theta_g}(x)}dG(x).
\end{aligned}$$

Here, $\mathscr{X}_j \equiv \mathscr{X}_{j,0} = \mathscr{X}_{j,\varepsilon}|_{\varepsilon=0}$, $j \in \{1,2\}$. Since, $\tau(x)+1 = \frac{G(x)}{F_\theta(x)}$ when $x \in \mathscr{X}_1$ and $\tau(x)+1 = \frac{\bar{G}(x)}{S_\theta(x)}$ when $x \in \mathscr{X}_2$, we get the required result.

When $G = F_\theta$ is the true distribution function, we have, $\theta_g = \theta$ and $\tau(x) = 0$. Noting $H(0) = 1$, $H'(0) = 0$ and substituting these values, we get the simple form of the influence function

$$T'(y) = \left[\int -\nabla u_\theta(x)dF_\theta(x)\right]^{-1} u_\theta(y) = I^{-1}(\theta)u_\theta(y),$$

which is the same as the influence function of the maximum likelihood estimator at the model. □

## 3 Location-Scale Equivariance

**Theorem 2** *The proposed weighted likelihood estimators are location-scale equivariant.*

*Proof* We have $Z_1, Z_2, \cdots, Z_n$ independent and identically distributed observations from a location-scale family with probability density function $\frac{1}{\sigma}f_{(0,1)}(\frac{x-\mu}{\sigma})$, parametrized by $(\mu,\sigma)$. We know that $(\hat{\mu},\hat{\sigma})$ are weighted likelihood estimators of $(\mu,\sigma)$ obtained form solving the equation

$$\frac{1}{n}\sum_{i=1}^{n} H(\tau^Z_{(\mu,\sigma)}(Z_i))u_{(\mu,\sigma)}(Z_i) = 0.$$

We intend to show that for $a \in \mathbb{R}$ and $b > 0$ and for $X_i = a + bZ_i$, $i = 1,2,\cdots,n$; $(a+b\hat{\mu}, b\hat{\sigma})$ will be the weighted likelihood estimators of $(a+b\mu, b\sigma)$.

In order to obtain the said estimators, we need to show

$$\frac{1}{n}\sum_{i=1}^{n} H(\tau^X_{(a+b\hat{\mu},b\hat{\sigma})}(X_i))u_{(a+b\hat{\mu},b\hat{\sigma})}(X_i) = 0.$$

We will show that for any choice of $a, \mu \in \mathbb{R}$, $b > 0, \sigma > 0$ and for any $z \in \mathbb{R}$ and $x = a + bz$,

$$H(\tau^X_{(a+b\mu,b\sigma)}(x)) = H(\tau^Z_{(\mu,\sigma)}(z)),$$
$$u_{(a+b\mu,b\sigma)}(x) = u_{(\mu,\sigma)}(z).$$

We first see that $F_{(a+b\mu,b\sigma)}(x) = F_{(\mu,\sigma)}(z)$ and $S_{(a+b\mu,b\sigma)}(x) = S_{(\mu,\sigma)}(z)$. Also note that,

$$F_n^Z(z) = \frac{1}{n}\sum_{i=1}^{n}\mathbf{1}_{\{Z_i\leqslant z\}} = \frac{1}{n}\sum_{i=1}^{n}\mathbf{1}_{\{X_i\leqslant x\}} = F_n^X(x),$$
$$S_n^Z(z) = \frac{1}{n}\sum_{i=1}^{n}\mathbf{1}_{\{Z_i\geqslant z\}} = \frac{1}{n}\sum_{i=1}^{n}\mathbf{1}_{\{X_i\geqslant x\}} = S_n^X(x).$$

Now, when $F_{(a+b\mu,b\sigma)}(x) = F_{(\mu,\sigma)}(z) \leqslant 1/2$ ,

$$\tau^X_{(a+b\mu,b\sigma)}(x) = \frac{F_n^X(x)}{F_{(a+b\mu,b\sigma)}(x)} - 1 = \frac{F_n^Z(z)}{F_{(\mu,\sigma)}(z)} - 1 = \tau^Z_{(\mu,\sigma)}(z).$$

Otherwise,

$$\tau^X_{(a+b\mu,b\sigma)}(x) = \frac{S_n^X(x)}{S_{(a+b\mu,b\sigma)}(x)} - 1 = \frac{S_n^Z(z)}{S_{(\mu,\sigma)}(z)} - 1 = \tau^Z_{(\mu,\sigma)}(z).$$

Note that the function $H(\cdot)$ is not inherently dependent on the parameter $\theta$, rather it is the residual function, which is the argument of $H(\cdot)$, that induces the dependence on $\theta$. Since we have $\tau^X_{(a+b\mu,b\sigma)}(x) = \tau^Z_{(\mu,\sigma)}(z)$, we can conclude

$$H(\tau^X_{(a+b\mu,b\sigma)}(x)) = H(\tau^Z_{(\mu,\sigma)}(z)).$$

As to show the equality of the score functions, we note that score function is simply the derivative of the natural logarithm of the corresponding probability density function with respect to the parameters. So, we now proceed to show the equality of the derivatives involved. Since we are dealing with a location-scale family, the probability density functions of $Z$ and $X$ are of the form

$$f_{(\mu,\sigma)}(z) = \frac{1}{\sigma}f_{(0,1)}\left(\frac{z-\mu}{\sigma}\right)$$

and

$$f_{(a+b\mu,b\sigma)}(x) = \frac{1}{b\sigma}f_{(0,1)}\left(\frac{x-a-b\mu}{b\sigma}\right) = \frac{1}{b\sigma}f_{(0,1)}\left(\frac{z-\mu}{\sigma}\right)$$

respectively. Taking natural logarithm we get,

$$\ln f_{(\mu,\sigma)}(z) = -\ln\sigma + \ln f_{(0,1)}\left(\frac{z-\mu}{\sigma}\right),$$
$$\ln f_{(a+b\mu,b\sigma)}(x) = -\ln b - \ln\sigma + \ln f_{(0,1)}\left(\frac{z-\mu}{\sigma}\right).$$

Since the two functions differ only by a constant (in this case $-\ln b$), their derivatives with respect to both $\mu$ and $\sigma$ will be the same, thereby assuring

$$u_{(a+b\mu,b\sigma)}(x) = u_{(\mu,\sigma)}(z).$$

Now that we have the two desired results, we see that

$$\frac{1}{n}\sum_{i=1}^{n}H(\tau^X_{(a+b\hat{\mu},b\hat{\sigma})}(X_i))u_{(a+b\hat{\mu},b\hat{\sigma})}(X_i) = \frac{1}{n}\sum_{i=1}^{n}H(\tau^Z_{(\hat{\mu},\hat{\sigma})}(Z_i))u_{(\hat{\mu},\hat{\sigma})}(Z_i) = 0.$$

Thus we complete the proof of the theorem. □

## 4 Consistency & Asymptotic Efficiency

### 4.1 Regularity Conditions

We first present some regularity conditions. While the general case involving multiple parameters can be handled by making the conditions more complicated and by routinely extending the proof, in the following we consider the case of a scalar parameter.

(C1) The weight function $H(\tau)$ is nonnegative, bounded above by 1 and twice differentiable with respect to $\tau$; $H(0) = 1$ and $H'(0) = 0$.

(C2) The function $H'(\tau)(1+\tau)$ is bounded, where $H'(\tau)$ is the derivative of $H(\tau)$ with respect to $\tau$.

(C3) The function $H''(\tau)(1+\tau)^2$ is bounded. Further, $H''(\tau)$ is continuous in $\tau$.

(C4) For every $\theta_0 \in \Theta$, there is a neighborhood $N(\theta_0)$ such that for every $\theta \in N(\theta_0)$, the quantities $|\tilde{u}_\theta(x)\nabla u_\theta(x)|$, $|\tilde{u}^2_\theta(x)u_\theta(x)|$, $|\nabla\tilde{u}_\theta(x)u_\theta(x)|$ and $|\nabla_2 u_\theta(x)|$ are bounded by $M_1(x), M_2(x), M_3(x)$ and $M_4(x)$ respectively, where $\nabla_2$ represents second derivative with respect to $\theta$ and $\mathbb{E}_{\theta_0}[M_i(X)] < \infty$ for $i = 1,2,3,4$.

(C5) $\mathbb{E}_{\theta_0}[\tilde{u}^2_\theta(X)u^2_\theta(X)] < \infty$ and $\mathbb{E}_{\theta_0}[(\nabla u_\theta)^2(X)] < \infty$.

(C6) The Fisher Information $I(\theta) = \mathbb{E}_\theta[u^2_\theta(X)]$ is nonzero, finite and positive for any $\theta \in \Theta$.

Here, $\tilde{u}_\theta(x)$ is defined as

$$\tilde{u}_\theta(x) = \begin{cases} \dfrac{\nabla F_\theta(x)}{F_\theta(x)}, & \text{if } 0 < F_\theta(x) \leqslant 1/2 \\ \dfrac{\nabla S_\theta(x)}{S_\theta(x)}, & \text{if } 1/2 < F_\theta(x) < 1. \end{cases}$$

All the proposed weight functions follow the conditions (C1) to (C3) and we assume the conditions (C4) to (C6) to be true.

### 4.2 Main Theorem for Consistency and Asymptotic Efficiency

**Theorem 3** *Let the true distribution belong to the model, $\theta_0$ be the true parameter and let $\hat{\theta}_{n,WLE}$ be the weighted likelihood estimator. Under conditions (C1) - (C6) the following results hold:*

1. *The convergence*

$$\sqrt{n}\left|A_n - \frac{1}{n}\sum_{i=1}^{n} u_{\theta_0}(X_i)\right| \to 0$$

*holds in probability, where $A_n = \frac{1}{n}\sum_{i=1}^{n} H(\tau_{n,\theta_0}(X_i))u_{\theta_0}(X_i)$, and $H(\tau_{n,\theta_0}(X_i))$ are weights based on the residual function $\tau_{n,\theta_0}(X_i)$ .*

2. *The convergence*

$$\left|B_n - \frac{1}{n}\sum_{i=1}^{n} \nabla u_{\theta_0}(X_i)\right| \to 0$$

*holds in probability, where $B_n = \frac{1}{n}\sum_{i=1}^{n} \nabla(w_\theta(\tau_{n,\theta_0}(X_i))u_\theta(X_i))\Big|_{\theta=\theta_0}$.*

3. *$C_n = O_p(1)$, where $C_n = \frac{1}{n}\sum_{i=1}^{n} \nabla_2(w_\theta(\tau_{n,\theta_0}(X_i))u_\theta(X_i))\Big|_{\theta=\theta'}$. Here $\theta'$ is in between $\theta_0$ and $\hat{\theta}_{n,WLE}$ and $\nabla_2$ represents second derivative with respect to $\theta$.*

### *4.2.1* Remarks and Necessary Corollaries

In the proof of the above theorem which follows shortly, we modify our residual functions slightly, such that the modified residual function is asymptotically same as the residual function we defined. We modify the residual function $\tau_{n,\theta}(\cdot)$ the following way

$$\tilde{\tau}_{n,k,\theta}(x) = \begin{cases} 0, & \text{if } 0 \leqslant F_\theta(x) \leqslant k^{-1}n^{-3/4} \\ \dfrac{F_n(x)}{F_\theta(x)} - 1 & \text{if } k^{-1}n^{-3/4} < F_\theta(x) \leqslant 1/2 \\ \dfrac{S_n(x)}{S_\theta(x)} - 1 & \text{if } 1/2 < F_\theta(x) \leqslant 1 - k^{-1}n^{-3/4} \\ 0, & \text{if } 1 - k^{-1}n^{-3/4} < F_\theta(x) \leqslant 1. \end{cases} \tag{8}$$

Apparently, this change in the definition may seem contrary to the idea conveyed in the original definition of the residual function. However, a residual equal to zero leads to a weight equal to 1, and if anything, makes the asymptotics easier. Also we may notice that while doing any real data analysis or simulation, we can always make the smallest observation fall outside this region by appropriately choosing the value of $k$ to ensure $k > \dfrac{1}{n^{3/4}F_{\theta_0}(\text{the minimum observation})}$. In particular, therefore, the use of the residual (8) makes no difference to our estimation scheme. To avoid further notational complications, we will continue to denote the residual function as $\tau_{n,\theta_0}(x)$ in the subsequent developments, but will actually use the residual function $\tilde{\tau}_{n,\theta_0}(x)$ defined in (8).

Having defined this new residual function, we will now proceed to establish the required results for the residual $\tilde{\tau}_{n,k,\theta}(\cdot)$ in place of $\tau_{n,\theta}(\cdot)$. To avoid cumbersome notations, we proceed with the notation $\tau_{n,\theta}(\cdot)$ although the residual function being implied is actually $\tilde{\tau}_{n,k,\theta}(\cdot)$.

*Remark 1* We have seen that for all fixed, positive values of $k$, the limiting distribution of $\tilde{\tau}_{n,k,\theta}(\cdot)$, as $n \to \infty$, remains same. The modified residual function $\tilde{\tau}_{n,k,\theta}(\cdot)$ has been introduced to avoid the unboundedness of $\tau_{n,\theta}(\cdot)$. The redefinition only affects the extreme tails in the $\tau$ scale, and the redefined residuals are smaller than $o_P(n^{-1/2})$ terms. For the purpose of simulation, we preassign large values of $k$.

Before beginning to prove the Theorem above, we present two very important Corollaries that are the focus of this text.

**Corollary 1** *There exists a sequence $\{\hat{\theta}_{n,WLE}\}_{n\in\mathbb{N}}$ of roots of the weighted likelihood estimating equation 2 such that*

$$\hat{\theta}_{n,WLE} \xrightarrow{P} \theta_0.$$

*Proof (Proof of Corollary:)* The proof essentially stems from the ideas introduced in Serfling (1980) and Lehmann and Casella (2006). We first generalize the notations used in Theorem 3. Let us define the following

$$A_n(\theta) = \frac{1}{n}\sum_{i=1}^{n} H(\tau_{n,\theta}(X_i))U_\theta(X_i,\Delta_i),$$

$$B_n(\theta) = \frac{1}{n}\sum_{i=1}^{n} \nabla\left(H(\tau_{n,\theta}(X_i))U_\theta(X_i,\Delta_i)\right), \text{ and}$$

$$C_n(\theta) = \frac{1}{n}\sum_{i=1}^{n} \nabla_2\left(H(\tau_{n,\theta}(X_i))U_\theta(X_i,\Delta_i)\right).$$

Clearly, $A_n \equiv A_n(\theta_0)$, $B_n \equiv B_n(\theta_0)$ and $C_n \equiv C_n(\theta_n')$, where $\theta_n'$ is some point lying on the line joining $\theta_0$ and $\hat{\theta}_{n,\text{WLE}}$.

The idea of the proof is that given any $\varepsilon > 0$, the root of the equation 2 lies inside the interval $(\theta_0 - \varepsilon, \theta_0 + \varepsilon)$. For this, following the line of Serfling (1980), we assert the following

*Claim* For any $\varepsilon > 0$,

$$\mathbb{P}_{\theta_0}\left[|A_n(\theta_0 - \varepsilon) - \varepsilon J(\theta_0)| > \frac{3}{4}\varepsilon J(\theta_0)\right] \longrightarrow 0, \text{ and}$$

$$\mathbb{P}_{\theta_0}\left[|A_n(\theta_0 + \varepsilon) + \varepsilon J(\theta_0)| > \frac{3}{4}\varepsilon J(\theta_0)\right] \longrightarrow 0.$$

*Proof (Proof of Claim:)* We show the first assertion. The second one follows in the same vein.

Now, a Taylor series expansion of the term $A_n(\theta_0-\varepsilon)$ around $\theta_0$ will produce

$$\begin{aligned}A_n(\theta_0-\varepsilon) &= A_n(\theta_0)+(-\varepsilon)B_n(\theta_0)+\frac{1}{2}\varepsilon^2 C_n(\theta')\\ &= A_n-\varepsilon B_n+\frac{1}{2}\varepsilon^2 C_n.\end{aligned}$$

Then,

$$\begin{aligned}&|A_n(\theta_0-\varepsilon)-\varepsilon J(\theta_0)|\\ =\ &|A_n-\varepsilon B_n+\frac{1}{2}\varepsilon^2 C_n-\varepsilon J(\theta_0)|\\ \leqslant\ &|A_n-\varepsilon(B_n+J(\theta_0))+\frac{1}{2}\varepsilon^2 C_n|\\ \leqslant\ &|A_n|+\varepsilon|B_n+J(\theta_0)|+\frac{1}{2}\varepsilon^2|C_n|.\end{aligned}$$

Thus, the first probability expression becomes

$$\begin{aligned}&\mathbb{P}_{\theta_0}\left[|A_n(\theta_0-\varepsilon)-\varepsilon J(\theta_0)|>\frac{3}{4}\varepsilon J(\theta_0)\right]\\ \leqslant\ &\mathbb{P}_{\theta_0}\left[|A_n|+\varepsilon|B_n+J(\theta_0)|+\frac{1}{2}\varepsilon^2|C_n|>\frac{3}{4}\varepsilon J(\theta_0)\right]\\ \leqslant\ &\mathbb{P}_{\theta_0}\left[|A_n|>\frac{1}{4}\varepsilon J(\theta_0)\right]+\mathbb{P}_{\theta_0}\left[\varepsilon|B_n+J(\theta_0)|>\frac{1}{4}\varepsilon J(\theta_0)\right]\\ &+\mathbb{P}_{\theta_0}\left[\frac{1}{2}\varepsilon^2|C_n|>\frac{1}{4}\varepsilon J(\theta_0)\right].\end{aligned}$$

From Theorem 3, we have,

$$A_n=o_P(1),\ \ B_n+J(\theta_0)=o_P(1) \text{ and } C_n=O_P(1).$$

Thus, each of the terms in the last inequality above approaches zero as $n\to\infty$. Hence the proof of the claim.

From the claim above, it follows that for any $\varepsilon>0$,

$$\mathbb{P}_{\theta_0}\left[A_n(\theta_0-\varepsilon)<0 \text{ and } A_n(\theta_0+\varepsilon)>0\right]\longrightarrow 1, \text{ as } n\longrightarrow\infty.$$

Thus, using the continuity of $A_n(\theta)$, we conclude that for any $\varepsilon>0$,
$\mathbb{P}_{\theta_0}\left[\exists \text{a root of 2 in the interval}(\theta_0-\varepsilon,\theta_0+\varepsilon)\right]\longrightarrow 1, \text{ as } n\longrightarrow\infty.$

Let us define this zero of $A_n(\theta)$ by

$$\hat{\theta}_{n,\mathrm{WLE}}(\varepsilon)=\inf\left\{\theta:\theta\in(\theta_0-\varepsilon,\theta_0+\varepsilon) \text{ and } A_n(\theta)=0\right\}.$$

The measurability of $\hat{\theta}_{n,\mathrm{WLE}}(\varepsilon)$ follows in the same line as illustrated in Serfling (1980). However, this root depends upon both $\theta_0$ (which is unknown) and $\varepsilon$. It can easily be seen that $\hat{\theta}_{n,\mathrm{WLE}}(\varepsilon)$ is consistent for $\theta_0$. Let us now illustrate one technique that has been adopted in order to avoid the dependencies of the root on $\theta_0$ and $\varepsilon$.

Let $\{T_n\}_{n\in\mathbb{N}}$ be a sequence of consistent estimators of $\theta_0$, which can be obtained under fairly general conditions. Let us define the following estimator.

$$\hat{\theta}_{n,\mathrm{WLE}}=\begin{cases}\text{The solution of 2 closest to } T_n, & \text{if } \exists \text{ at least one solution}\\ \theta_1\in\Theta, \text{arbitrary}, & \text{if } \exists \text{ no solution.}\end{cases}$$

Employing this technique, we achieve a sequence $\{\hat{\theta}_{n,\mathrm{WLE}}\}$ of consistent solutions of 2 and complete the proof. □

**Corollary 2** $\sqrt{n}(\hat{\theta}_{n,WLE}-\theta_0)\xrightarrow{\mathscr{D}} N(0,J^{-1}(\theta_0))$.

*Proof (Proof of Corollary:)* Expanding the left side of 2 at $\theta = \hat{\theta}_{n,\text{WLE}}$ about the true parameter $\theta_0$ results in

$$\sqrt{n}(\hat{\theta}_{n,\text{WLE}} - \theta_0) = -\frac{\sqrt{n}A_n}{B_n + \frac{(\hat{\theta}_{n,\text{WLE}} - \theta_0)}{2} C_n}.$$

Now, from Theorem 3, we get,

$$\sqrt{n}A_n \xrightarrow{\mathscr{D}} N(0, J(\theta_0)).$$

Also, from Corollary 1, $(\hat{\theta}_{n,\text{WLE}} - \theta_0) = o_P(1)$ and $C_n = O_P(1)$. So, $(\hat{\theta}_{n,\text{WLE}} - \theta_0)C_n = o_P(1)$. Hence, we conclude

$$\sqrt{n}(\hat{\theta}_{n,\text{WLE}} - \theta_0) \xrightarrow{\mathscr{D}} N(0, J^{-1}(\theta_0)).$$

□

### *4.2.2* **Proof of Main Theorem**

*Proof (Proof of Theorem 3)* For proving the first result, we do a Taylor series expansion of $H(\tau_{n,\theta_0}(X_i))$ around 0 which gives

$$H(\tau_{n,\theta_0}(X_i)) - 1 = H(0) + H'(0)\tau_{n,\theta_0}(X_i) + \frac{H''(\xi_i)}{2}\tau^2_{n,\theta_0}(X_i) - 1.$$

From the given conditions, $H(0) = 1, H'(0) = 0$ and $|H''(x)| \leqslant K_0$ for some large enough $K_0 > 0$ and for all $x \in [-1, \infty)$. Using these facts, we establish that

$$\{H(\tau_{n,\theta_0}(X_i)) - 1\}^2 \leqslant K_0^2 \tau^4_{n,\theta_0}(X_i)/4.$$

We now proceed to calculate the expected value of $\{H(\tau_{n,\theta_0}(X_i)) - 1\}^2$. Clearly,

$$\mathbb{E}_{\theta_0}\left[(H(\tau_{n,\theta_0}(X_i)) - 1)^2\right] \leqslant K_0^2 \mathbb{E}_{\theta_0}(\tau^4_{n,\theta_0}(X_i))/4.$$

To calculate the above, we notice that

$$\mathbb{E}\left[\tau^4_{n,\theta_0}(X_i)\right] = \mathbb{E}\left[\mathbb{E}(\tau^4_{n,\theta_0}(X_i)|X_i = x)\right].$$

Since $X_1, X_2, \cdots, X_n$ are supposed to be i.i.d. observations coming from a continuous distribution, conditioning by $\{X_i = x\}$ is equivalent to conditioning by $\{F_{\theta_0}(X_i) = F_{\theta_0}(x)\}$.

It is to be noted here that for each $i$, $nF_n(X_i) - 1$ is a binomial random variable with parameters $(n-1)$ and $p_x = F_{\theta_0}(x)$ and $nS_n(X_i) - 1$ is another binomial random variable with parameters $(n-1)$ and $q_x = (1 - p_x) = 1 - F_{\theta_0}(x)$, conditional on $X_i = x$. Using the above result, we proceed to compute $E(\tau^4_{n,\theta_0}(X_i))$.

Let us first define the following subsets of $\mathscr{X}$

$$\begin{aligned}
\mathscr{X}_1 &= \left[F_{\theta_0}^{-1}(0), F_{\theta_0}^{-1}\left(\frac{1}{kn^{3/4}}\right)\right], \\
\mathscr{X}_2 &= \left(F_{\theta_0}^{-1}\left(\frac{1}{kn^{3/4}}\right), F_{\theta_0}^{-1}\left(\frac{1}{2}\right)\right], \\
\mathscr{X}_3 &= \left(F_{\theta_0}^{-1}\left(\frac{1}{2}\right), F_{\theta_0}^{-1}\left(1 - \frac{1}{kn^{3/4}}\right)\right], \\
\mathscr{X}_4 &= \left(F_{\theta_0}^{-1}\left(1 - \frac{1}{kn^{3/4}}\right), F_{\theta_0}^{-1}(1)\right].
\end{aligned}$$

Clearly, $\mathscr{X} = \bigcup_{j=1}^4 \mathscr{X}_j$. We will be evaluating $\mathbb{E}_{\theta_0}[\tau^4_{n,\theta_0}(X)]$ over these subsets separately.

For $x \in \mathscr{X}_2$, we have,

$$\begin{aligned}
\mathbb{E}_{\theta_0}[\tau^4_{n,\theta_0}(X_1)\mathbf{1}_{\{X_1\in\mathscr{X}_2\}}] &= \int_{\mathscr{X}_2} \mathbb{E}\left(\frac{F_n(X_1)-F_{\theta_0}(X_1)}{F_{\theta_0}(X_1)}\bigg|X_1=x\right)^4 dF_{\theta_0}(x)\\
&= \int_{\mathscr{X}_2} \frac{1}{n^4F^4_{\theta_0}(x)}\mathbb{E}\left[\{(nF_n(x)-1)+n(1-F_{\theta_0}(x))\}^4|X_1=x\right]dF_{\theta_0}(x)\\
&= \int_{\mathscr{X}_2} \frac{1}{n^4F^4_{\theta_0}(x)}\mathbb{E}\left[\{(nF_n(x)-1)-(n-1)F_{\theta_0}(x)+(1-F_{\theta_0}(x))\}^4|X_1=x\right]dF_{\theta_0}(x)\\
&= \int_{\mathscr{X}_2} \frac{1}{(np)^4}\mathbb{E}\left[\{(nF_n(x)-1)-(n-1)p+(1-p)\}^4|F_{\theta_0}(X_1)=p\right]dp
\end{aligned}$$

Due to symmetry in the expression of the asymptotic variance of $F_n$ and $S_n$, it can similarly be shown that

$$\mathbb{E}_{\theta_0}[\tau^4_{n,\theta_0}(X)\mathbf{1}_{\{X\in\mathscr{X}_2\cup\mathscr{X}_3\}}] \approx O(n^{-5/4}).$$

For subsets $\mathscr{X}_1$ and $\mathscr{X}_4$, it evidently follows that

$$\mathbb{E}_{\theta_0}[\tau^4_{n,\theta_0}(X)\mathbf{1}_{\{X\in\mathscr{X}_1\cup\mathscr{X}_4\}}] = 0.$$

Hence, we establish that

$$\mathbb{E}\left[H(\tau_{n,\theta_0}(X_i))-1\right]^2 \leqslant \frac{K_1}{n^{5/4}},$$

for an appropriate choice of $K_1$, depending on $k$.

Having established this, we now have,

$$\begin{aligned}
\mathbb{E}\left|(H(\tau_{n,\theta_0}(X_i))-1)u_{\theta_0}(X_i)\right| &\leqslant \mathbb{E}\left[(H(\tau_{n,\theta_0}(X_i))-1)^2\right]^{1/2}\mathbb{E}\left[u^2_{\theta_0}(X_i)\right]^{1/2}\\
&\leqslant \frac{K_2}{n^{5/8}},
\end{aligned}$$

for some $K_2$, depending on $k$. Hence,

$$\begin{aligned}
\mathbb{E}\left|\frac{1}{\sqrt{n}}\sum_{i=1}^n(H(\tau_{n,\theta_0}(X_i))-1)u_{\theta_0}(X_i)\right| &\leqslant \frac{1}{\sqrt{n}}\sum_{i=1}^n\mathbb{E}\left|(H(\tau_{n,\theta_0}(X_i))-1)u_{\theta_0}(X_i)\right|\\
&\leqslant \frac{1}{\sqrt{n}}\sum_{i=1}^n\frac{K_2}{n^{5/8}}\\
&= \frac{K_2}{n^{1/8}}\\
&\to 0.
\end{aligned}$$

Thus, we prove that

$$\sqrt{n}\left|A_n-\frac{1}{n}\sum_{i=1}^n u_{\theta_0}(X_i)\right| \xrightarrow{L_1} 0$$

and hence

$$\sqrt{n}\left|A_n-\frac{1}{n}\sum_{i=1}^n u_{\theta_0}(X_i)\right| \xrightarrow{P} 0.$$

This completes the proof of part 1.

We now proceed to prove part 2. Using an approach similar to the proof of part 1, we get,

$$\begin{aligned}
\left|B_n-\frac{1}{n}\sum_{i=1}^n\nabla u_{\theta_0}(X_i)\right| &\leqslant \frac{1}{n}\sum_{i=1}^n\left|H'(\tau_{n,\theta_0}(X_i))(1+\tau_{n,\theta_0}(X_i))\tilde{u}_{\theta_0}(X_i)u_{\theta_0}(X_i)\right|\\
&+\frac{1}{n}\sum_{i=1}^n\left|(H(\tau_{n,\theta_0}(X_i))-1)\nabla u_{\theta_0}(X_i)\right|.
\end{aligned}$$

We shall show that both the dominating terms go to 0 in probability. For the second term on the right, we already know that

$$\mathbb{E}\left[(H(\tau_{n,\theta_0}(X_i))-1)^2\right] \leqslant \frac{K_1}{n^{5/4}},$$

and as per our assumption, $\mathbb{E}\left[(\nabla u_{\theta_0})^2(X_i)\right]$ is finite. Combining these, we get,

$$\mathbb{E}\left[\frac{1}{n}\sum_{i=1}^{n}\left|(H(\tau_{n,\theta_0}(X_i))-1)\nabla u_{\theta_0}(X_i)\right|\right] \leqslant \frac{K_3}{n^{5/8}},$$

for some $K_3$ depending on $k$. Thus it leads to the conclusion that

$$\frac{1}{n}\sum_{i=1}^{n}\left|(H(\tau_{n,\theta_0}(X_i))-1)\nabla u_{\theta_0}(X_i)\right| \xrightarrow{P} 0.$$

In order to show convergence of the first term, we take a Taylor series expansion of $H'(\tau_{n,\theta_0}(X_i))$ around 0 to get

$$H'(\tau_{n,\theta_0}(X_i)) = H'(0) + \tau_{n,\theta_0}(X_i)H''(\xi_i),$$

where $\xi_i$ is in between 0 and $\tau_{n,\theta_0}(X_i)$. Since $H'(0)=0$ and $|H''(\xi_i)| \leqslant \tilde{K}$ for some appropriately chosen $\tilde{K}>0$, we have,

$$\mathbb{E}\left[(H'(\tau_{n,\theta_0}(X_i))(1+\tau_{n,\theta_0}(X_i)))^2\right] \leqslant \tilde{K}^2\mathbb{E}(\tau^2_{n,\theta_0}(X_i)+2\tau^3_{n,\theta_0}(X_i)+\tau^4_{n,\theta_0}(X_i)).$$

As before, we proceed to compute this expected value and see that the leading term is again of the order $n^{-5/4}$ and exactly like before, we have,

$$\frac{1}{n}\sum_{i=1}^{n}\left|H'(\tau_{n,\theta_0}(X_i))(1+\tau_{n,\theta_0}(X_i))\tilde{u}_{\theta_0}(X_i)u_{\theta_0}(X_i)\right| \leqslant \frac{K_4}{n^{5/8}}$$

for some $K_4>0$. And thus, this convergence also holds in probability. This yields

$$\left|B_n - \frac{1}{n}\sum_{i=1}^{n}\nabla u_{\theta_0}(X_i)\right| \xrightarrow{P} 0.$$

In order to prove the result regarding the third term, note that

$$\begin{aligned}
C_n &= \frac{1}{n}\sum_{i=1}^{n}\nabla_2(H(\tau_{n,\theta}(X_i))u_\theta(X_i))|_{\theta=\theta'} \\
&= \frac{1}{n}\sum_{i=1}^{n}H(\tau_{n,\theta'}(X_i))\nabla_2 u_{\theta'}(X_i) \\
&\quad -\frac{2}{n}\sum_{i=1}^{n}H'(\tau_{n,\theta'}(X_i))(1+\tau_{n,\theta'}(X_i))\tilde{u}_{\theta'}(X_i)\nabla u_{\theta'}(X_i) \\
&\quad -\frac{1}{n}\sum_{i=1}^{n}H'(\tau_{n,\theta'}(X_i))(1+\tau_{n,\theta'}(X_i))\nabla\tilde{u}_{\theta'}(X_i)u_{\theta'}(X_i) \\
&\quad +\frac{1}{n}\sum_{i=1}^{n}H'(\tau_{n,\theta'}(X_i))(1+\tau_{n,\theta'}(X_i))\tilde{u}^2_{\theta'}(X_i)u_{\theta'}(X_i) \\
&\quad +\frac{1}{n}\sum_{i=1}^{n}H''(\tau_{n,\theta'}(X_i))(1+\tau_{n,\theta'}(X_i))^2\tilde{u}^2_{\theta'}(X_i)u_{\theta'}(X_i).
\end{aligned}$$

Now, owing to the consistency of $\hat{\theta}_{\text{WLE}}$, for large enough $n$, we can choose a neighbourhood of $\theta_0$ which contains $\theta'$. Hence, under the assumption (A3), each of the terms in the right side is bounded. Thus, we conclude that

$$C_n = O_P(1)$$

and this completes the proof of the theorem. □

*Remark 2* $F_\theta(\cdot)$ is a function of $\theta$ and we assume it to be twice differentiable with respect to $\theta$. $\tau_{n,\theta}$ is a function of $F_\theta(\cdot)$. $\tilde{\tau}_{n,k,\theta}$ is a modification of $\tau_{n,\theta}$, changing it beyond certain constant (given n) values. $\tilde{\tau}_{n,k,\theta}$ may not be differentiable with respect to $\theta$ at (only) $F_\theta(x) = k^{-1}n^{-3/4}$ and $1-k^{-1}n^{-3/4}$. To bypass this inconvenience, let us define $\hat{\tau}_{n,k,\theta}$ in the following way:

$$\hat{\tau}_{n,k,\theta}(x) = \begin{cases} 0, & \text{if } 0 \leqslant F_\theta(x) \leqslant k^{-1}n^{-3/4}, \\ t_{n,\theta}(x), & \text{if } k^{-1}n^{-3/4} < F_\theta(x) \leqslant k^{-1}n^{-3/4} + \delta_n, \\ \dfrac{F_n(x)}{F_\theta(x)} - 1, & \text{if } k^{-1}n^{-3/4} + \delta_n < F_\theta(x) \leqslant 1/2, \\ \dfrac{S_n(x)}{S_\theta(x)} - 1, & \text{if } 1/2 < F_\theta(x) \leqslant 1 - k^{-1}n^{-3/4} - \delta_n, \\ s_{n,\theta}(x), & \text{if } 1 - k^{-1}n^{-3/4} - \delta_n < F_\theta(x) \leqslant 1 - k^{-1}n^{-3/4}, \\ 0, & \text{if } 1 - k^{-1}n^{-3/4} < F_\theta(x) \leqslant 1, \end{cases}$$

where $t_{n,\theta}(x)$ and $s_{n,\theta}(x)$ are functions such that the first and second derivative of $\hat{\tau}_{n,k,\theta}$ both exist and the choice of $\delta_n$ is made in such a way, that the ensuing changes do not affect the "in probability convergence" results.

## 5 Second Order Influence Function Analysis of the Estimator

**Theorem 4** *For the proposed weighted likelihood estimator,*

$$\theta''_\varepsilon\big|_{\varepsilon=0} = T''(y) = D_0^{-1}[(T'(y))^2 N_1 + 2T'(y)N_2 + N_3], \tag{9}$$

*where*

$$D_0 = \int H(\tau)\nabla u_\theta dG - \int_{\mathscr{X}_1} H'(\tau)u_\theta(\Delta_y - G)\frac{\nabla F_\theta}{F_\theta^2}dG - \int_{\mathscr{X}_2} H'(\tau)u_\theta(\bar{\Delta}_y - \bar{G})\frac{\nabla S_\theta}{S_\theta^2}dG,$$

$$\begin{aligned} N_1 = {} & 2\int_{\mathscr{X}_1} H'(\tau)\nabla u_\theta(\tau+1)\frac{\nabla F_\theta}{F_\theta}dG + \int_{\mathscr{X}_2} H'(\tau)\nabla u_\theta(\tau+1)\frac{\nabla S_\theta}{S_\theta}dG \\ & - \int_{\mathscr{X}_1} H''(\tau)u_\theta(\tau+1)^2\left(\frac{\nabla F_\theta}{F_\theta}\right)^2 F_\theta dG - \int_{\mathscr{X}_2} H''(\tau)u_\theta(\tau+1)^2\left(\frac{\nabla S_\theta}{S_\theta}\right)^2 S_\theta dG \\ & - \int_{\mathscr{X}_1} H'(\tau)u_\theta(\tau+1)\left[2\left(\frac{\nabla F_\theta}{F_\theta}\right)^2 - \frac{\nabla_2 F_\theta}{F_\theta}\right]dG \\ & - \int_{\mathscr{X}_2} H'(\tau)u_\theta(\tau+1)\left[2\left(\frac{\nabla S_\theta}{S_\theta}\right)^2 - \frac{\nabla_2 S_\theta}{S_\theta}\right]dG - \int H(\tau)\nabla_2 u_\theta dG, \end{aligned}$$

$$\begin{aligned} N_2 = {} & \int_{\mathscr{X}_1} H'(\tau)u_\theta(\tau+1)\frac{\nabla F_\theta}{F_\theta}dG + \int_{\mathscr{X}_2} H'(\tau)u_\theta(\tau+1)\frac{\nabla S_\theta}{S_\theta}dG \\ & - \int_{\mathscr{X}_1} H'(\tau)\nabla u_\theta\frac{\Delta_y - G}{F_\theta}dG - \int_{\mathscr{X}_2} H'(\tau)\nabla u_\theta\frac{\bar{\Delta}_y - \bar{G}}{S_\theta}dG \\ & + \int_{\mathscr{X}_1} H'(\tau)u_\theta(\Delta_y - G)\frac{\nabla F_\theta}{F_\theta^2}dG + \int_{\mathscr{X}_2} H'(\tau)u_\theta(\bar{\Delta}_y - \bar{G})\frac{\nabla S_\theta}{S_\theta^2}dG \\ & + \int_{\mathscr{X}_1} H''(\tau)u_\theta\frac{\nabla F_\theta}{F_\theta}(\tau+1)(\Delta_y - G)dG + \int_{\mathscr{X}_2} H''(\tau)u_\theta\frac{\nabla S_\theta}{S_\theta}(\tau+1)(\bar{\Delta}_y - \bar{G})dG \\ & - \int H(\tau)\nabla u_\theta d\Delta_y + \int H(\tau)\nabla u_\theta dG, \end{aligned}$$

$$N_3 = -\int_{\mathscr{X}_1} H''(\tau)\frac{u_\theta}{F_\theta}[\Delta_y - G]^2 dG - \int_{\mathscr{X}_2} H''(\tau)\frac{u_\theta}{S_\theta}[\bar{\Delta}_y - \bar{G}]^2 dG$$
$$-2\int_{\mathscr{X}_1} H'(\tau)u_\theta\frac{\Delta_y - G}{F_\theta}d(\Delta_y - G) - 2\int_{\mathscr{X}_2} H'(\tau)u_\theta\frac{\bar{\Delta}_y - \bar{G}}{S_\theta}d(\Delta_y - G).$$

*Proof* As before in Section 2.2, we denote $T(G_\varepsilon) = \theta_\varepsilon$ for a parametric family governed by the scalar parameter $\theta$. Let $\tau_\varepsilon$ be as defined in Section 2. Our estimating equation is

$$\int_{\mathscr{X}} H(\tau_\varepsilon(x))u_{\theta_\varepsilon}(x)dG_\varepsilon(x) = 0.$$

Successive differentiation of the estimating equation with respect to $\varepsilon$ gives,

$$\begin{aligned}
&\int_{\mathscr{X}} H''(\tau_\varepsilon)(\tau'_\varepsilon)^2 u_{\theta_\varepsilon} dG + \int_{\mathscr{X}} H'(\tau_\varepsilon)\tau''_\varepsilon u_{\theta_\varepsilon} dG \\
&+ \theta'_\varepsilon \int_{\mathscr{X}} H'(\tau'_\varepsilon)\tau'_\varepsilon \nabla u_{\theta_\varepsilon} dG + \int_{\mathscr{X}} H'(\tau_\varepsilon)\tau'_\varepsilon u_{\theta_\varepsilon} d(\Delta_y - G) \\
&+ \theta''_\varepsilon \int_{\mathscr{X}} H(\tau_\varepsilon)\nabla u_{\theta_\varepsilon} dG + \theta'_\varepsilon \int_{\mathscr{X}} H'(\tau_\varepsilon)\tau'_\varepsilon \nabla u_{\theta_\varepsilon} dG \\
&+ (\theta'_\varepsilon)^2 \int_{\mathscr{X}} H(\tau_\varepsilon)\nabla_2 u_{\theta_\varepsilon} dG + \theta'_\varepsilon \int_{\mathscr{X}} H(\tau_\varepsilon)\nabla u_{\theta_\varepsilon} d(\Delta_y - G) \\
&+ \int_{\mathscr{X}} H'(\tau_\varepsilon)\tau'_\varepsilon u_{\theta_\varepsilon} d(\Delta_y - G) + \theta'_\varepsilon \int_{\mathscr{X}} H(\tau_\varepsilon)\nabla u_{\theta_\varepsilon} d(\Delta_y - G) = 0.
\end{aligned}$$

We plug in the values of $\tau'_\varepsilon(x)$ and $\tau''_\varepsilon(x)$ in the above equation.

$$\tau'_\varepsilon(x) = \frac{1}{F_{\theta_\varepsilon}(x)}\left[\Delta_y(x) - G(x) - (\tau_\varepsilon + 1)\nabla F_{\theta_\varepsilon}(x)\theta'_\varepsilon\right]$$

or,

$$\tau'_\varepsilon(x) = \frac{1}{S_{\theta_\varepsilon}(x)}[\bar{\Delta}_y(x)^* - \bar{G}^*(x) - (\tau_\varepsilon + 1)\nabla S_{\theta_\varepsilon}(x)\theta'_\varepsilon]$$

according to whether $x \in \mathscr{X}_{1,\varepsilon}$ or $x \in \mathscr{X}_{2,\varepsilon}$. And,

$$\begin{aligned}
\tau''_\varepsilon =& 2(\tau_\varepsilon + 1)\left(\frac{\nabla F_{\theta_\varepsilon}}{F_{\theta_\varepsilon}}\right)^2 (\theta'_\varepsilon)^2 - 2\frac{(\Delta_y - G)}{F_{\theta_\varepsilon}}\frac{\nabla F_{\theta_\varepsilon}}{F_{\theta_\varepsilon}}\theta'_\varepsilon \\
&- (\tau_\varepsilon + 1)\frac{\nabla_2 F_{\theta_\varepsilon}}{F_{\theta_\varepsilon}}(\theta'_\varepsilon)^2 - (\tau_\varepsilon + 1)\frac{\nabla F_{\theta_\varepsilon}}{F_{\theta_\varepsilon}}\theta''_\varepsilon
\end{aligned}$$

or,

$$\begin{aligned}
\tau''_\varepsilon =& 2(\tau_\varepsilon + 1)\left(\frac{\nabla S_{\theta_\varepsilon}}{S_{\theta_\varepsilon}}\right)^2 (\theta'_\varepsilon)^2 - 2\frac{(\bar{\Delta}^*_y - \bar{G})}{S_{\theta_\varepsilon}}\frac{\nabla S_{\theta_\varepsilon}}{S_{\theta_\varepsilon}}\theta'_\varepsilon \\
&- (\tau_\varepsilon + 1)\frac{\nabla_2 S_{\theta_\varepsilon}}{S_{\theta_\varepsilon}}(\theta'_\varepsilon)^2 - (\tau_\varepsilon + 1)\frac{\nabla S_{\theta_\varepsilon}}{S_{\theta_\varepsilon}}\theta''_\varepsilon
\end{aligned}$$

according to whether $x \in \mathscr{X}_{1,\varepsilon}$ or $x \in \mathscr{X}_{2,\varepsilon}$.

Plugging these values and after a simple although tedious manipulation, we get,

$$\theta''_\varepsilon\big|_{\varepsilon=0} = T''(y) = D_0^{-1}[(T'(y))^2 N_1 + 2T'(y)N_2 + N_3], \tag{10}$$

where

$$D_0 = \int H(\tau)\nabla u_\theta dG - \int_{\mathscr{X}_1} H'(\tau)u_\theta(\Delta_y - G)\frac{\nabla F_\theta}{F_\theta^2}dG - \int_{\mathscr{X}_2} H'(\tau)u_\theta(\bar{\Delta}_y - \bar{G})\frac{\nabla S_\theta}{S_\theta^2}dG,$$

$$
\begin{aligned}
N_1 = {} & 2\int_{\mathscr{X}_1} H'(\tau)\nabla u_\theta(\tau+1)\frac{\nabla F_\theta}{F_\theta}dG + \int_{\mathscr{X}_2} H'(\tau)\nabla u_\theta(\tau+1)\frac{\nabla S_\theta}{S_\theta}dG \\
& - \int_{\mathscr{X}_1} H''(\tau)u_\theta(\tau+1)^2\left(\frac{\nabla F_\theta}{F_\theta}\right)^2 F_\theta dG - \int_{\mathscr{X}_2} H''(\tau)u_\theta(\tau+1)^2\left(\frac{\nabla S_\theta}{S_\theta}\right)^2 S_\theta dG \\
& - \int_{\mathscr{X}_1} H'(\tau)u_\theta(\tau+1)\left[2\left(\frac{\nabla F_\theta}{F_\theta}\right)^2 - \frac{\nabla_2 F_\theta}{F_\theta}\right] dG \\
& - \int_{\mathscr{X}_2} H'(\tau)u_\theta(\tau+1)\left[2\left(\frac{\nabla S_\theta}{S_\theta}\right)^2 - \frac{\nabla_2 S_\theta}{S_\theta}\right] dG - \int H(\tau)\nabla_2 u_\theta dG,
\end{aligned}
$$

$$
\begin{aligned}
N_2 = {} & \int_{\mathscr{X}_1} H'(\tau)u_\theta(\tau+1)\frac{\nabla F_\theta}{F_\theta}dG + \int_{\mathscr{X}_2} H'(\tau)u_\theta(\tau+1)\frac{\nabla S_\theta}{S_\theta}dG \\
& - \int_{\mathscr{X}_1} H'(\tau)\nabla u_\theta\frac{\Delta_y - G}{F_\theta}dG - \int_{\mathscr{X}_2} H'(\tau)\nabla u_\theta\frac{\bar{\Delta}_y - \bar{G}}{S_\theta}dG \\
& + \int_{\mathscr{X}_1} H'(\tau)u_\theta(\Delta_y - G)\frac{\nabla F_\theta}{F_\theta^2}dG + \int_{\mathscr{X}_2} H'(\tau)u_\theta(\bar{\Delta}_y - \bar{G})\frac{\nabla S_\theta}{S_\theta^2}dG \\
& + \int_{\mathscr{X}_1} H''(\tau)u_\theta\frac{\nabla F_\theta}{F_\theta}(\tau+1)(\Delta_y - G)dG + \int_{\mathscr{X}_2} H''(\tau)u_\theta\frac{\nabla S_\theta}{S_\theta}(\tau+1)(\bar{\Delta}_y - \bar{G})dG \\
& - \int H(\tau)\nabla u_\theta d\Delta_y + \int H(\tau)\nabla u_\theta dG,
\end{aligned}
$$

$$
\begin{aligned}
N_3 = {} & -\int_{\mathscr{X}_1} H''(\tau)\frac{u_\theta}{F_\theta}[\Delta_y - G]^2 dG - \int_{\mathscr{X}_2} H''(\tau)\frac{u_\theta}{S_\theta}[\bar{\Delta}_y - \bar{G}]^2 dG \\
& -2\int_{\mathscr{X}_1} H'(\tau)u_\theta\frac{\Delta_y - G}{F_\theta}d(\Delta_y - G) - 2\int_{\mathscr{X}_2} H'(\tau)u_\theta\frac{\bar{\Delta}_y - \bar{G}}{S_\theta}d(\Delta_y - G).
\end{aligned}
$$

□

## References

Lehmann EL, Casella G (2006) Theory of point estimation. Springer Science & Business Media
Serfling RJ (1980) Approximation Theorems of Mathematical Statistics. John Wiley & Sons, New York
